# Supplementary material for: AutoPhoto: Aesthetic Photo Capture using Reinforcement Learning
Source: arXiv:2109.09923 source file (2021-09-21)
Supplement: Supplementary file 1 [file appendix.tex]

\hadi{we do set a hard limit of 100 steps in both training and eval -- forgot to mention that in the paper. Is here the best place to mention it? Is it important to mention it? median num. of steps is significantly less}

    % Alternative captions for table 3
    % because the aesthetics model is only an approximation of human preferences.}
    
    % Human users also consistently prefer the photos from AutoPhoto over the random initial views. The aesthetic model is only an approximation of human preferences so the agreement between the aesthetic model and human users is not perfect.  \hadi{@Hubert: this last sentence does the trick? should we move it earlier}}
    % \hubert{Maybe place human prefs on left, model prefs on right. Frame as: AutoPhoto trained with aesthetics model as oracle. Aesthetics model likes autophoto output XX\% of the time. However, aesthetic model is approximation of human preferences. We see that real humans also consistently prefer autophoto outputs over random starting locations.} We assess the aesthetic quality of the photos captured by our method against the photos of the starting views, by comparing their aesthetic scores and by collecting users' preferences. The performance with respect to the aesthetic model is fairly consistent across simulated scenes like in Gibson and Matterpot3D and real life photos, with a small drop in performance, even though the model wasn't trained on real scenes. We also see that users tend to consider the photos that our system output better than the initial view, which shows that our system can capture well-composed photos in simulation and real life that agrees with user preferences.}
